# Supplementary material for: Nanowire growth and sublimation: CdTe quantum dots in ZnTe nanowires
Source: arXiv:1803.10610 source file (2018-04-13)
Supplement: Supplementary file 1 [file Orru_Supp.pdf]

## Supplementary material

## Nanowire growth and sublimation: CdTe quantum dots in ZnTe nanowires

M. Orrù,[†,‡] E. Robin,[‡] M. Den Hertog,[†] K. Moratis,[†] Y. Genuist,[†]
R. André,[†] D. Ferrand,[†] J. Cibert, [†] and E. Bellet-Amalric [‡]

[†] Univ. Grenoble Alpes, CNRS, Institut NEEL, F-38000 Grenoble, France,
[‡] Univ. Grenoble Alpes, CEA, INAC, F-38000 Grenoble, France

# Thermodynamics of Cd in Au

We summarize here the data available on the behavior of Cd in the gold-assisted growth of CdTe nanowires and dots embedded in nanowires: (1) the Cd vapor pressure and the activity of Cd in solid Au, which governs the evaporation of Cd from the nanoparticle; (2) the diffusion of Cd in Au and its modification by finite-size effects.

### 1. Cd vapor pressure

#### a. Pure Cd

The vapor pressure above pure Cd is well documented, and the differences between different formulae are not significant for the present purpose. We use, for liquid Cd, $\log p_{Cd}(T) = 10.248 - 5392/T$, units Pa and K, *i.e.*, $p_{Cd}(T) = p_0 \exp(-\frac{12416}{T})$ with $p_0 = 1.770 \times 10^{10}$ Pa and an activation energy 1.07 eV [1]. At 350°C, *T*=623K, the calculated pressure is $p_{Cd}$ =39 Pa.

#### b. Solid solution of Cd in Au

Cd forms a solid solution with Au, up to values of the concentration *c* at which well-identified phase transitions are observed. The Cd partial pressure $p_{Cd}(c,T)$ above the solid solution has been measured for temperatures *T* slightly larger than ours, around 1000K in Ref. 2 and 550°C (823K) in Ref. 3. Both plot the value of the activity $a(c,T) = p_{Cd}(c,T)/p_{Cd}(T)$, parametrized as $\log a = A + \frac{B}{T}$, for fixed values of *c* above 8%; they report quite small values of $a$ at low concentration, with $\frac{a}{c} \ll 1$, increasing regularly with *c*. We use the low-*c* data of Ref 3 as they feature less scattering and the temperature range is closer to ours.

We have to deal however with even smaller values of *c*. At vanishingly low Cd content, the limit should obey the regular solution model for an alloy with two components. In this model the Gibbs free energy *G* of a solid solution of cadmium in gold is expressed using the free energy $G_{Cd}$ of pure Cd and $G_{Au}$ of pure Au, the so-called interaction parameter Ω (representing the difference of bond energies), and the ideal entropy $k_B \ln c$. With $n_{Au}$ the number of Au atoms and $n_{Cd}$ that of Cd, so that $c = n_{Cd}/(n_{Au} + n_{Cd})$, the free energy is written

$$G = n_{Au}G_{Au} + n_{Cd}G_{Cd} + \frac{n_{Au}n_{Cd}}{n_{Au}+n_{Cd}}\Omega + k_B T\left[n_{Au}\ln\frac{n_{Au}}{n_{Au}+n_{Cd}} + n_{Cd}\ln\frac{n_{Cd}}{n_{Au}+n_{Cd}}\right],$$

and the chemical potential is

$\mu_{Cd} = \frac{\partial G}{\partial n_{Cd}} = G_{Cd} + (1-c)^2\Omega + k_B T \ln c$; the activity follows as

$$k_B T \ln a(c,T) = (1-c)^2\Omega + k_B T \ln c.$$

The interaction parameter Ω is expected [4] to depend smoothly on *T* and *c*. In a finite range of temperature, we can develop $\Omega(T) \approx \Omega_0 + \Omega_1 k_B T$, so that

$$k_B T \ln a(c,T) = (1-c)^2\Omega_0 + k_B T(\Omega_1 + \ln c).$$

According to Eq. 4 of Ref. 4, Ω contains the concentration *c* only in a denominator, which is equal to $\left(1 + c\frac{V_{Cd}-V_{Au}}{V_{Au}}\right)$, where $V_{Cd}$ ($V_{Au}$) is the molar volume of Cd (resp. Au). Using the density of Cd and Au (8.65 and 19.3) and their atomic weight (112.4 and 197), we get $\frac{V_{Cd}-V_{Au}}{V_{Au}}$=0.27. Thus we obtain the activity as $k_B T \ln a(c,T) = \frac{(1-c)^2}{1+0.27c}\Omega_0 + k_B T(\Omega_1 + \ln c)$, to be used to fit the usual parametrization $\log a = A + \frac{B}{T}$. Indeed the thermodynamic quantities at 550°C tabulated in Ref. 3 as a function of *c* are reasonably well fitted by this expression assuming constant values of $\Omega_0$ and $\Omega_1$ (not shown). Finally, the direct fit of *A* and *B* results in $a_{Cd} = 2.8\, c \exp\left(-7800\frac{(1-c)^2}{1+0.27c}\frac{1}{T}\right)$, see Fig. S1.

Finally our best estimate is (in Pa)

$$p_{Cd}(c,T) = 4.96 \times 10^{10}\, c \exp\left[-\frac{1}{T}\left(12416 + 7800\frac{(1-c)^2}{1+0.27c}\right)\right].$$

### 2. Diffusion in a Cd-Au alloy.

Two sets of data are available on the diffusion of Cd in gold.

- The diffusion coefficient has been measured by PIXE (proton induced x-ray emission) for temperatures above 750°C and Cd content of a few %.[5] A typical value is $D = 10^{-9}$ cm$^2$ s$^{-1}$ at 1023K (750°C). The uncertainty on the activation energy is high. It is noticed that in this temperature range the diffusion of Cd in Au is much larger than the self-diffusion of Au, $\frac{D_{Cd}}{D_{Au}} \approx 8$, the lighter the faster [5].
- The analysis of the deposition rate of Cd on Au through electrodeposition around room temperature is interpreted [6,7] as involving the diffusion of Cd in bulk Au, with $D \approx 10^{-18}$ cm$^2$ s$^{-1}$. However the actual value unexpectedly depends on the applied bias, and the interpretation needs to invoke another, faster contribution close to the surface. A strong

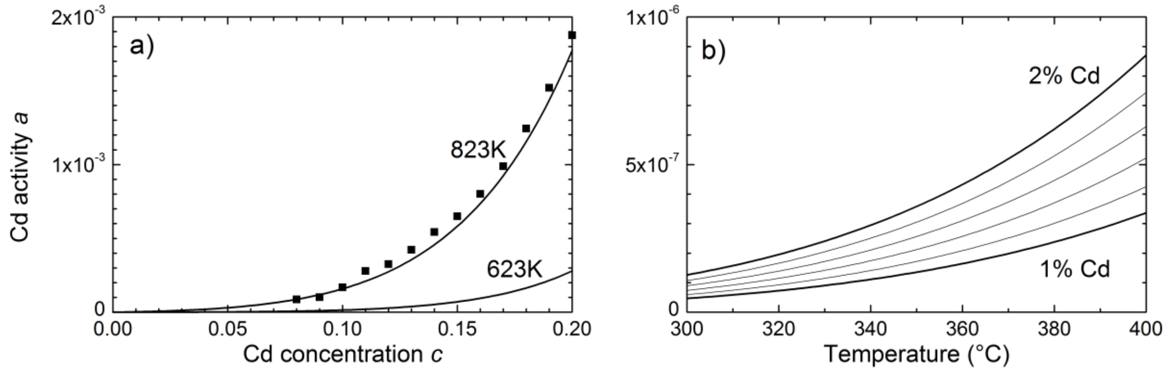


**Figure S1.** (a) Activity of Cd in gold, as a function of concentration. Symbols are data from Ref. 3, the upper solid line is our fit using the regular solution model, calculated at 823 K, and the lower one the extrapolation to 623 K; (b) temperature dependence for the same model extrapolated to low values of the concentration, as indicated.

enhancement of the diffusion was also reported in the case of Zn in Au-nanoparticles.[8]

Interpolating with an Arrhenius law between these two sets of data, we obtain $D \approx 10^{-12}$ cm$^2$ s$^{-1}$ at 350°C.

The flux $j_{\mathrm{Cd}}$ to carry under the present growth conditions of nanowires is 0.5 ML s$^{-1}$ of (001) CdTe, or 0.5 Cd atom per ${a_0}^2/2$ with $a_0 = 0.648$ nm for CdTe; hence $j_{\mathrm{Cd}} = 2 \times 10^{14}$ cm$^{-2}$ s$^{-1}$. If this is associated to the diffusion of Cd through the Au nanoparticle, assuming a concentration difference smaller than $\Delta c = 1\%$ over the height $h$=5 nm of the nanoparticle, $j_{\mathrm{Cd}} = D \frac{\Delta c}{h} \frac{4}{{a_0}^3}$ (where the gold atom volume is 4/$a_0^3$ with $a_0$ = 0.41 nm for Au), leading to $D > 10^{-13}$ cm$^2$ s$^{-1}$. This is one order of magnitude below the previously interpolated value. Hence the mechanism of diffusion through the nanoparticle is not unrealistic, even if some atoms go through the surface or its vicinity and if the details should be taken into account in a complete model of the CdTe growth.

### 3. Finite size effects.

In the frame of the ZnTe nanowire growth, the gold nanoparticle generally assumes the shape of a half-sphere or a full sphere [9], with a diameter around 15 to 25 nm, although facets are occasionally identified [10]. The surface energy of gold is calculated [11] to be $\gamma \approx$1.5 J m$^{-2}$, with a small dependence on orientation; hence we expect an influence from the Gibbs-Thomson effect on the chemical potential of Cd in the nanoparticle, $\Delta\mu = \frac{2\gamma}{R} \approx 0.94$ eV nm$^{-3}$, or 16 meV / atom (taking the volume of gold as 1.7×10$^{-2}$ nm$^3$ corresponding to a weight 197 g mol$^{-1}$, and a density 19.3×10$^6$ g/m$^3$). This is not completely negligible compared to $k_B T$ and to the chemical potential of the ideal alloy and should be taken into account in a complete description of the nanowire growth.

When the impinging flux is stopped, the evaporation tends to decrease the Cd content until it stops; at the same time dissolution of the CdTe nanowire maintains a higher concentration $c$ in the vicinity of the nanowire-nanoparticle interface. The result is a gradient of concentration $\nabla c$ (and a gradient of chemical potential $\nabla\mu$) along the axis. The response to this gradient is a current of Cd atoms, $j_{Cd} = D_{Cd}\, \nabla c\, \frac{4}{{a_0}^3}$, from the interface towards the apex of the nanoparticle, and the equilibrium is reached when the Cd gradient is such that the dissolution current, the evaporation current, and the diffusion current $j$ are balanced.

The concentration gradient induces also a current of Au atoms, $j_{Au} = D_{Au}\, \nabla(1-c)\, \frac{4}{{a_0}^3}$, which is much smaller. Through the Gibbs-Thomson effect, the bulb shape creates a uniform term which opposes the gradient of chemical potential $\nabla\mu$ for Cd, as discussed in the main text.

**References**


[1] David R. Lide (ed), CRC Handbook of Chemistry and Physics, 84th Edition, online version. CRC Press. Boca Raton, Florida, **2003**; Section 4, Properties of the Elements and Inorganic Compounds; Vapor Pressure of the Metallic Elements.

[2] J. D. Filby and J. N. Pratt, Trans. Faraday Soc. **60**, 1934 (1964).

[3] L. J. Bartha and W. A. Alexander, Can. J. Chem. **43**, 2319 (1965).

[4] F. Glas,J. Appl. Phys. **108**, 073506 (2010).

[5] D. Decroupet, and G. Demortier, Nuclear Inst. Methods in Phys. B, **49**, 501 (1990).

[6] Ruxandra Vidu and Shigeta Hara, Surface Sci. **452**, 229 (2000).

[7] Tomofumi Tanaka Kimihiko Kubo Nobumitsu Hirai, and Shigeta Hara; Materials transactions, **44**, 688 (2003).

[8] H. Yasuda and H. Mori, Phys. Rev. Lett. **69**, 3747 (1992).

[9] P. Rueda-Fonseca, M. Orrù, E. Bellet-Amalric, E. Robin, M. Den Hertog, Y. Genuist, R. André, S. Tatarenko, and J. Cibert, J. Appl. Phys. **119**, 164303 (2016).

[10] P. Rueda-Fonseca, E. Bellet-Amalric, R. Vigliaturo, M. Den Hertog, Y. Genuist, R. André, E. Robin, A. Artioli, P. Stepanov, D. Ferrand, K. Kheng, S. Tatarenko, and J. Cibert, Nano Lett. **14**, 1877 (2014).

[11] L. Vitos, A.V. Ruban, H.L. Skriver, J. Kollár, Surface Sci. **411**, 186 (1998).
